# Supplementary material for: Automated Discovery of Process Models from Event Logs: Review and Benchmark
Source: arXiv:1705.02288 source file (2018-01-30)
Supplement: Supplementary file 1 [file appendix.tex]

%\section{Appendix}
%\label{appendix}

\begin{comment}
\begin{landscape}% Landscape page
\centering
\begin{table}
\begin{adjustbox}{width=1.5\textwidth,center=\textwidth}
\pgfplotstabletypeset[
%column type=l,
every head row/.style={
before row={%
\toprule
\multicolumn{1}{c}{\textbf{Id}} & \multicolumn{1}{c}{\textbf{Name}} & \multicolumn{1}{c}{\textbf{Authors}} & \multicolumn{1}{c}{\textbf{Year}} & %\multicolumn{5}{c}{\textbf{Taxonomy}} &
\multicolumn{1}{c}{\textbf{Model Type}} & \multicolumn{1}{c}{\textbf{Model language}} &  \multicolumn{5}{c}{\textbf{Process constraints}} & \multicolumn{1}{c}{\textbf{Implementation}} & \multicolumn{3}{c}{\textbf{Evaluation}} & \multicolumn{1}{c}{\textbf{Available?}}\\
},
after row=\midrule,
},
every last row/.style={
after row=\bottomrule},
columns/person/.style ={column name=},
columns/extra/.style ={column name=},
columns/authors/.style ={column name=},
columns/year/.style ={column name=},
%columns/freqHeur/.style ={column name=\(H_{freq}\)},
%columns/genHeur/.style ={column name=\(H_{gen}\)},
%columns/regions/.style ={column name=\(T_{reg}\)},
%columns/probabilistic/.style ={column name=Probabilistic},
%columns/others/.style ={column name=Other},
columns/modtype/.style ={column name=},
columns/langClass/.style ={column name=},
columns/para/.style ={column name=AND},
columns/exclusive/.style ={column name=XOR},
columns/or/.style ={column name=OR},
columns/loop/.style ={column name=Cycle},
columns/declare/.style ={column name=Declare},
columns/imple/.style ={column name=},
columns/evReal/.style ={column name=Real-life},
columns/evSynth/.style ={column name=Synthetic},
columns/evArt/.style ={column name=Artificial},
columns/forFree/.style ={column name=},
%columns/assessed/.style ={column name=},
col sep=&,row sep=\\,
string type,
]{
person & extra  & authors & year & modtype & langClass & para & exclusive & or & loop & declare & imple & evReal & evSynth & evArt & forFree \\
% S1 & Fuzzy Map Miner & Li et al.\cite{li2010mining} & 2011 & Procedural & Fuzzy maps &  & \checkmark &  & \checkmark & & ProM & \checkmark &  &  & \checkmark \\
 S2 & Process Spaceship & Motahari et al.\cite{motahari2011event} & 2011 & Procedural & State machines & \checkmark & \checkmark &  & \checkmark & & Eclipse & \checkmark & \checkmark & &\checkmark \\
% S3 & Event Cube & Ribeiro and Weijters\cite{ribeiro2011event} & 2011 & Procedural & Dependency graphs & \checkmark & \checkmark & \checkmark & \checkmark & & ProM & & & \checkmark & \checkmark \\
 S4 & HK & Huang and Kumar\cite{huang2012study} & 2012 & Procedural & Petri nets & \checkmark & \checkmark & & \checkmark & & Standalone & \checkmark & \checkmark & &  \\
% S5 & ProCube & van der Aalst\cite{van2013process} & 2013 & Multi & Multi & \checkmark & \checkmark &  & \checkmark & & ProM &  & & &\checkmark  \\
 %S6 & MailOfMine & Di Ciccio, Mecella\cite{di2013mining} & 2013 & Declarative & Declare & & & & & \checkmark & Standalone & \checkmark & \checkmark &  & \checkmark  \\
 %S8 & passages-based ILP Miner & Verbeek et al.\cite{verbeek2012experimental} & 2013 & Procedural & Petri nets & \checkmark & \checkmark & & \checkmark & & ProM & \checkmark & & \checkmark & \checkmark \\
% S9 & Data-flow Discovery & De Leoni, van der Aalst\cite{de2013data} & 2013 & Procedural & Petri nets & \checkmark & \checkmark & & \checkmark & & ProM & \checkmark & \checkmark &  & \checkmark \\
% S10 & Inductive Miner & Leemans et al.\cite{leemans2013discovering} & 2013 & Procedural & Process trees& \checkmark & \checkmark &  & \checkmark  & & ProM &  &  & \checkmark & \checkmark \\
 S11 & Declare Miner & Maggi et al.\cite{DBLP:conf/caise/MaggiBA12} & 2012 & Declarative & Declare & & & & & \checkmark & ProM & \checkmark & \checkmark  &  & \checkmark \\
 S7 & MINERful & Di Ciccio, Mecella\cite{di2013two} & 2013 & Declarative & Declare & & & & & \checkmark & ProM, Standalone & \checkmark  & \checkmark &  & \checkmark\\
 S18 & Inductive Miner - Infrequent & Leemans et al.\cite{DBLP:conf/bpm/LeemansFA13} & 2013 & Procedural & Process trees & \checkmark & \checkmark & \checkmark & \checkmark & & ProM & \checkmark &  &  & \checkmark \\
 S17 & Runtime Process Skeletonization & Abe, Kudo\cite{abe2014business} & 2014 & Procedural & Fuzzy maps & & \checkmark &  & \checkmark & & Standalone & \checkmark &  &  &  \\
 S20 & ETM & Buijs\cite{buijs2014quality} & 2014 & Procedural & Process trees & \checkmark & \checkmark & \checkmark &\checkmark  & & ProM & \checkmark &  & \checkmark & \checkmark \\
 S21 & Updated Heuristics Miner & De Cnudde et al.\cite{de2014improving} & 2014 & Procedural & BPMN & \checkmark & \checkmark &  & \checkmark & & ProM & \checkmark &  & \checkmark & \\
 S12 & WoMan & Ferilli\cite{ferilli2014woman} & 2014 & Declarative & WoMan & & & & & \checkmark & Standalone & \checkmark &  & \checkmark &  \\
% S13 & hierarchical approach & Arbab et al.\cite{arbab2014hierarchical} & 2014 & Procedural & HMM model & \checkmark & \checkmark &  & \checkmark & & Standalone & \checkmark & & &  \\
 S14 & HybridMiner & Maggi et al.\cite{maggi2014automated} & 2014 & Hybrid & Declare + Petri nets & \checkmark & \checkmark &  & \checkmark & \checkmark & ProM & \checkmark &  &  & \checkmark\\
 S22 & Competition Miner %Dynamic Constructs Comptetition Miner 
     & Redlich et al.\cite{redlich2014dynamic} & 2014 & Procedural & BPMN & \checkmark & \checkmark &  & \checkmark & & Standalone & \checkmark & & & \\
 S15 & DAG & Vasilecas et al.\cite{vasilecas2014directed} & 2014 & Procedural & DAG & & \checkmark &  & & & Standalone & \checkmark & \checkmark &  & \\
 S33 & Decomposed Process Miner %Discover with ILP using Decomposition 
     & Verbeek, van der Aalst\cite{verbeek2014decomposed} & 2014 & Procedural & Petri nets & \checkmark & \checkmark & \checkmark & \checkmark & & ProM & \checkmark &  &  & \checkmark \\
% S19 & Inductive Miner - Incompleteness & Leemans et al.\cite{leemans2014discovering} & 2014 & Procedural & Process trees & \checkmark & \checkmark &  & \checkmark & & ProM &  &  & \checkmark & \checkmark\\
% S23 & BoR & Bleser et al.\cite{bleser2015cognitive} & 2015 & Procedural & HMM models & \checkmark & \checkmark &  &  \checkmark & & Standalone & \checkmark &  &  &\\
% S25 & Inductive visual Miner & Leemans et al.\cite{leemans2014exploring} & 2015 & PN+BPMN parallel GW & \checkmark & \checkmark &  & \checkmark & & ProM & \checkmark &  &  & \checkmark\\
% S27 & ArtifactModeling & Popova et al.\cite{popova2015artifact} & 2015 & Procedural & Guard-Stage-Milestone notation & & &  & & & ProM & \checkmark  & & & \checkmark\\
% S28 & Episode Miner & Leemans, van der Aalst\cite{leemans2014discovery2} & 2015 & Procedural & Episodes &  &  &  &  & & ProM & \checkmark &  & \checkmark & \checkmark\\
 S29 & MVPM Mine & Folino et al.\cite{folino2015discovery} & 2015 & Procedural & Heuristics nets & & \checkmark &  & \checkmark & & Standalone & \checkmark & & & \\
 S31 & CNMining & Greco et al.\cite{greco2015process} & 2015 & Procedural & Causal nets & \checkmark & \checkmark &  & \checkmark & & ProM & \checkmark & \checkmark & & \checkmark \\
 S30 & $\alpha$\$ & Guo et al.\cite{guo2015mining} & 2015 & Procedural & Petri nets & \checkmark & \checkmark &  & \checkmark & & ProM & \checkmark &  & \checkmark & \checkmark\\
 S32 & Maximal Pattern Mining & Liesaputra et al.\cite{liesaputra2015efficient} & 2015 & Procedural & Workflow net & \checkmark & \checkmark &  & \checkmark & & ProM & \checkmark & & \checkmark & \\
 %S34 & MINERful & Di Ciccio et al.\cite{di2015ensuring} & 2015 & Declarative & Declare & & & & & \checkmark & ProM, Standalone & \checkmark &  &  & \checkmark\\
% S35 & OLAPDiscovery & Pizarro, Sep\'{u}lveda\cite{pizarro2014experimenting} & 2015 & Multi & Social network, heuristic net & \checkmark & \checkmark &  & \checkmark & & ProM & \checkmark &  &  & \checkmark\\
 S36 & Supervised Polyhedra & Ponce de Leon et al.\cite{ponce2015incorporating} & 2015 & Procedural & Petri nets & \checkmark & \checkmark &  & \checkmark & & Standalone & \checkmark &  &  & \\
% S38 & IMD framework & Leemans et al.\cite{leemans2015scalable, leemansscalable} & 2015,2016 & Procedural & process tree, PN & \checkmark & \checkmark &  & \checkmark & & ProM & \checkmark &  & \checkmark & \checkmark\\
 S40 & DGEM & Molka et al.\cite{molka2015diversity} & 2015 & Procedural & BPMN & \checkmark & \checkmark &  & \checkmark & & Standalone & \checkmark & & \checkmark &\\
 S37 & LocalizedLogs & van der Aalst et al.\cite{van2015process} & 2015 & Procedural & Petri nets & \checkmark & \checkmark &  & \checkmark & & ProM & \checkmark & \checkmark &  & \checkmark\\
 S39 & HybridILPMiner & van Zelst et al.\cite{van2015ilp} & 2015 & Procedural & Petri nets & \checkmark & \checkmark &  & \checkmark & & ProM &  &  & \checkmark & \checkmark\\
 S26 & ProDiGen & Vazguez et al.\cite{vazquez2015prodigen} & 2015 & Procedural & Heuristics nets & \checkmark & \checkmark &  & \checkmark & & Standalone &  & \checkmark & \checkmark & \\
% S41 & Causality Miner & Ladiges et al.\cite{ladiges2015learning} & 2016 & Procedural & Petri nets & \checkmark & \checkmark &  & \checkmark & & Standalone & \checkmark &  &  &\\
 S43 & Structured Miner & Augusto et al.\cite{augusto2016automated} & 2016 & Procedural & BPMN & \checkmark & \checkmark &  & \checkmark & & ProM, Standalone & & \checkmark & \checkmark & \checkmark\\
 S55 & Non-Atomic Declare Miner & Bernardi et al.\cite{bernardi2016activity} & 2016 & Declarative & Declare & & & & & \checkmark & ProM & \checkmark & \checkmark &  & \checkmark \\
 S42 & RegPFA & Breuker et al.\cite{breuker2016comprehensible} & 2016 & Procedural & Petri nets & \checkmark & \checkmark &  & \checkmark & & Standalone & \checkmark & \checkmark & & \checkmark\\
 S16 & BPMNMiner & Conforti et al.\cite{conforti2016bpmn} & 2016 & Procedural & BPMN & \checkmark & \checkmark & \checkmark & \checkmark & & ProM, Apromore & \checkmark & & \checkmark & \checkmark \\
 S53 & TB-MINERful & Di Ciccio et al.\cite{di2016efficient} & 2016 & Declarative & Declare & & & & & \checkmark & Standalone &  \checkmark &  & \checkmark & \\
% S44 & Local & Tax et al.\cite{tax2016mining} & 2016 & Procedural & Process trees & \checkmark & \checkmark &  & \checkmark & & Standalone & \checkmark & & &\\
 S47 & PGminer & Mokhov et al.\cite{mokhov2016mining} & 2016 & Procedural & Partial Order Graphs %Conditional Partial Order Graphs 
     & \checkmark & \checkmark &  & & & Workcraft, Standalone & \checkmark & & \checkmark & \checkmark\\
 S45 & SQLMiner & Sch\"{o}nig et al.\cite{schonig2016efficient} & 2016 & Declarative & Declare & & &  & & \checkmark & Standalone & \checkmark &  &  & \checkmark \\
 S24 & ProM-D & Song et al.\cite{song2016process} & 2016 & Procedural & Petri nets & \checkmark & \checkmark & & \checkmark & & Standalone & \checkmark & \checkmark & & \\
% S46 & TM & Srinivasan et al.\cite{srinivasan2015identification} & 2016 & Procedural & Petri nets & \checkmark & \checkmark &  & \checkmark & & Standalone &  & \checkmark &  & \\
% S48 & MINERful-vacuityCheck & Maggi et al.\cite{maggi2016semantical} & 2016 & Declarative & Declare & & & & & \checkmark & Standalone & \checkmark &  &  & \checkmark \\
 S49 & CSMMiner & van Eck et al.\cite{van2016discovering} & 2016 & Procedural & State machines & \checkmark & \checkmark &  & \checkmark & & ProM & \checkmark & & & \checkmark \\
% S50 & Log OnMap Replayer & de Leoni et al.\cite{de2013turning} & 2016 & Procedural & multi & \checkmark & \checkmark &  & \checkmark & & ProM & \checkmark &  &  & \checkmark \\
 S51 & Proximity Miner & Yahya et al.\cite{yahya2016domain} & 2016 & Procedural & Heuristic nets & \checkmark & \checkmark &  & \checkmark & & ProM & \checkmark &  &  & \checkmark \\
% S52 & IMLC & Leemans et al.\cite{leemans2015using} & 2016 & Procedural & process tree, PN & \checkmark & \checkmark &  & \checkmark & & ProM &  &  & \checkmark & \checkmark\\
% S54 & MapReduce & Evermann\cite{evermann2014scalable} & 2016 & Procedural & Heuristics nets & \checkmark & \checkmark &  & \checkmark & & Standalone &  & \checkmark & & \\
}
\end{adjustbox}
\\ \\
\caption{Overview of the 32 discovery approaches identified (\{year, author\} ordered).}
\label{tab:SumTabel}
\end{table}
\end{landscape}

%S45 & SQLMiner & Schönig et al.\cite{schonig2016efficient} & 2016 & \checkmark & & & &  & Declarative & Declare & \checkmark & \checkmark &  & \checkmark & Standalone & \checkmark &  &  & \checkmark \\
%\scriptsize$^{***}$ Finds Declare constraints, but doesn't visualize them.\newline

%$^{*}$ Block-structure models, similar to restricted Petri net with invisible tasks
% S4 & HK & Huang and Kumar\cite{huang2012study} & 2012 & & & & & \checkmark & Procedural & Petri net$^{*}$ & \checkmark & \checkmark & & \checkmark & Standalone & \checkmark & \checkmark & &  \\

%$^{**}$ Mines models similar to the Fuzzy maps.
% S17 & Runtime process skeletonization & Abe, Kudo\cite{abe2014business} & 2014 & \checkmark & & & &  & Procedural & Fuzzy map$^{**}$ & \checkmark & \checkmark &  & \checkmark & Standalone & \checkmark &  &  &  \
\end{comment}
